# Supplementary material for: Effect of the avoided crossing on the rovibrational energy levels, resonances, and predissociation lifetimes within the ground and first excited electronic states of lithium fluoride
Source: arXiv:2512.02085 ancillary file (2025-12-01)
Supplement: Supplementary file 1 [file Resonances_and_Derivatives.pdf]

**Supplementary file “Resonances”: Additional notes on the calculation of the positions and widths of the resonances**

1. Out of all the resonances found, we select only narrow ones, with  $\Gamma_J < 1 \text{ cm}^{-1}$ . For  $r_{\text{max}} = 15 \text{ \AA}$  used by us, neglecting the first term in the right-hand side of Eq. (64) is justified.
2. The eigenvalues of energy,  $E$ , found by the sinc-DVR method do not coincide with true positions of the resonances,  $E_J$ . If the difference appreciably exceeds the width of the resonance, the resonant third term in Eq. (64) decreases and can become comparable with the first one, in which case the calculation of the position and width of the resonance by Eqs. (73)-(74) loses its accuracy. Therefore, at a given  $r_{\text{max}}$ , we select only those resonances that satisfy condition  $\delta E < \Gamma_J$ ; an additional requirement must be fulfilled that the energy difference between the current resonance and the neighboring non-resonant states be larger than  $10\Gamma_J$ .

It is possible that some resonances are not found by such a procedure. Yet, the resonance lost can appear at a different value of  $r_{\text{max}}$ . Therefore, we increase  $r_{\text{max}}$  by  $0.1 \text{ \AA}$  and repeat the procedure until no new resonances are discovered after at least five repetitions. On average, two or three lost resonances are discovered, and usually five to ten such iterations (and diagonalizations of the Hamiltonian matrix) are needed.

With use of the procedure described above, the most of the resonances will be discovered many times at different values of  $r_{\text{max}}$ , the positions and widths of one and the same resonance being somewhat (insignificantly) different for various  $r_{\text{max}}$ . As a final result, we select the one with the smallest value of the width,  $\Gamma_J$ .

In the final variant, the following procedure was used.

1. Select the value of  $r_{\text{max}} = 15 \text{ \AA}$  and find the eigenvalues of energy, *i.e.* diagonalize the Hamiltonian matrix.
2. For each level with the energy above the dissociation limit,  $E > 0$ , we find the energy derivatives over  $r_{\text{max}}$  and the values of  $\delta E$  and  $\Gamma_J$  by Eqs. (69)-(71). The resonant states are those with  $\Gamma_J \leq 1.2 \text{ cm}^{-1}$  and for which  $E'$  calculated by Eq. (76) is 2.5 times larger than the resonance value.
3. Refine step by step the positions and widths of the resonances with  $|\delta E|/\Gamma_J > 0.1$ . To this end, shift  $r_{\text{max}}$  by such  $\delta r_{\text{max}}$  that the boundary condition (64) be fulfilled at  $E = E_J$ . The required  $\delta r_{\text{max}}$  is found from Eq. (63),

$$\delta r_{\text{max}} = \frac{1}{k} \begin{cases} +\frac{\pi}{2} - \arctan(\Gamma_J/2\delta E), & \delta E > 0, \\ -\frac{\pi}{2} - \arctan(\Gamma_J/2\delta E), & \delta E < 0 \end{cases} \quad (80)$$

As a result, the value of  $|\delta E|/\Gamma_J$  decreases by orders of magnitude, thereby refining the position and width of the resonance under consideration. Other resonances also change their values of  $|\delta E|/\Gamma_J$ . If the new value turns out to decrease, replace the previous values of the parameters with the new ones. Sometimes, new resonances appear because a resonance

that did not fulfil the selection requirements at the first step can fulfil them at the new value of  $r_{\max}$ .

4. Repeat the refining procedure until all the resonances found have  $|\delta E|/\Gamma_J < 0.1$ . Typically, this requires about ten matrix diagonalizations at different values of  $r_{\max}$  described above.
5. Finally, out of all the resonances thus found, select only those ones with  $\Gamma_J \leq 1 \text{ cm}^{-1}$ .

The procedures described above apply only to the states with energies  $E \leq 7800 \text{ cm}^{-1}$  since, at higher energies, the outer turning point in the Coulomb potential approaches our value of  $r_{\max} = 15 \text{ \AA}$ .

**Supplementary file “Derivatives”: Calculation of the energy derivatives**

$\mathcal{H}$ , the Hamiltonian matrix including the DVR matrix of the kinetic energy, the rotational energy, the diabatic potential energies, and the nonadiabatic corrections.

$\mathbf{U}$ , the orthogonal matrix diagonalizing the Hamiltonian matrix,

$$\mathbf{U}^T \mathcal{H} \mathbf{U} = \mathbf{E}, \quad (81)$$

where  $\mathbf{E}$  is diagonal matrix of the eigenvalues of energy. The following relations are fulfilled:

$$\mathcal{H} = \mathcal{H}^T \quad (82)$$

$$\mathbf{U}^T \mathbf{U} = \mathbf{U} \mathbf{U}^T = \mathbf{I} \quad (83)$$

$$\mathcal{H} \mathbf{U} = \mathbf{U} \mathbf{E}, \quad \mathbf{U}^T \mathcal{H} = \mathbf{E} \mathbf{U}^T, \quad (84)$$

Let us determine matrix  $\mathbf{S}$ ,

$$\mathbf{S} = (\mathbf{U}')^T \mathbf{U}, \quad \mathbf{S}^T = \mathbf{U}^T \mathbf{U}'. \quad (85)$$

Taking the derivative of Eq. (83), we find

$$\mathbf{S} + \mathbf{S}^T = 0 \quad (86)$$

Thus, the diagonal elements of this matrix vanish.

By differentiating Eq. (81) and using the above relations. we obtain step by step

$$\mathbf{E}' = (\mathbf{U}')^T \mathcal{H} \mathbf{U} + \mathbf{U}^T \mathcal{H} \mathbf{U}' + \mathbf{U}^T \mathcal{H}' \mathbf{U}, \quad (87)$$

$$\mathbf{E}' = (\mathbf{U}')^T \mathbf{U} \mathbf{E} + \mathbf{E} \mathbf{U}^T \mathbf{U}' + \mathbf{U}^T \mathcal{H}' \mathbf{U}, \quad (88)$$

$$\mathbf{E}' = \mathbf{S} \mathbf{E} + \mathbf{E} \mathbf{S}^T + \mathbf{U}^T \mathcal{H}' \mathbf{U}, \quad (89)$$

$$\mathbf{E}' = \mathbf{S} \mathbf{E} - \mathbf{E} \mathbf{S} + \mathbf{U}^T \mathcal{H}' \mathbf{U}. \quad (90)$$

Matrix  $\mathbf{A}$ ,

$$\mathbf{A} = \mathbf{S} \mathbf{E} - \mathbf{E} \mathbf{S}, \quad (91)$$

is symmetric and has zeros at its diagonal (easy to verify),

$$\mathbf{A}^T = \mathbf{A}, \quad \mathbf{A}_{nn} = 0. \quad (92)$$

Therefore, as seen from Eq. (90), the derivatives of the energy eigenvalues are equal to the diagonal elements of matrix  $\mathbf{U}^T \mathcal{H}' \mathbf{U}$ ,

$$E'_n = (\mathbf{U}^T \mathcal{H}' \mathbf{U})_{nn} \quad (93)$$

or, explicitly,

$$E'_n = \sum_{i,k} \mathcal{H}'_{ik} U_{in} U_{kn} \quad (94)$$

We obtain from Eq. (90)

$$\mathbf{S}\mathbf{E} - \mathbf{E}\mathbf{S} + \mathbf{M} = 0, \quad (95)$$

where

$$M_{ik} = \begin{cases} (\mathbf{U}^T \mathcal{H}' \mathbf{U})_{ik}, & i \neq k, \\ 0, & i = k. \end{cases} \quad (96)$$

The same Eq. (95) in the matrix elements,

$$S_{ik}E_k - E_iS_{ik} + M_{ik} = 0. \quad (97)$$

Thus,

$$S_{ik} = \frac{M_{ik}}{E_i - E_k}, \quad i \neq k \quad (98)$$

Remind that the diagonal elements of  $\mathbf{S}$  are equal to zero. From Eq. (85), we find the derivatives of the eigenvectors (wavefunctions),

$$\mathbf{U}' = \mathbf{U} \mathbf{S}^T, \quad (99)$$

*i.e.*,

$$U'_{ik} = \sum_{j \neq k} U_{ij} \frac{M_{kj}}{E_k - E_j}. \quad (100)$$

Taking the derivative of Eq. (94), we obtain

$$E''_n = \sum_{i,k} (\mathcal{H}''_{ik} U_{in} U_{kn} + 2\mathcal{H}'_{ik} U'_{in} U_{kn}), \quad (101)$$

the second term in the sum being

$$\begin{aligned} \sum_{i,k} \mathcal{H}'_{ik} U'_{in} U_{kn} &= \sum_{i,k,j \neq n} \mathcal{H}'_{ik} U_{ij} \frac{M_{nj}}{E_n - E_j} U_{kn} \\ &= \sum_{j \neq n} \frac{M_{jn} M_{nj}}{E_n - E_j}. \end{aligned} \quad (102)$$

Finally,

$$E''_n = \sum_{i,k} \mathcal{H}''_{ik} U_{in} U_{kn} + 2 \sum_{j \neq n} \frac{M_{jn} M_{nj}}{E_n - E_j} \quad (103)$$

(note that  $M_{jn} = M_{nj}$ ).
